# Supplementary material for: Normalized topological indices discriminate between architectures of branched macromolecules
Source: arXiv:2409.16007 source file (2025-05-16)
Supplement: Supplementary file 1 [file SI.pdf]

# SUPPORTING INFORMATION:

# Normalized topological indices discriminate between architectures of branched macromolecules

Domen Vaupotič
*Department of Theoretical Physics, Jožef Stefan Institute, Ljubljana, Slovenia and Faculty of Mathematics and Physics, University of Ljubljana, Ljubljana, Slovenia*

Jules Morand
*Department of Civil, Environmental and Mechanical Engineering, University of Trento, Trento, Italy and INFN-TIFPA, Trento Institute for Fundamental Physics and Applications, Trento, Italy*

Luca Tubiana
*Department of Physics, University of Trento, Trento, Italy and INFN-TIFPA, Trento Institute for Fundamental Physics and Applications, Trento, Italy*

Anže Božič*
*Department of Theoretical Physics, Jožef Stefan Institute, Ljubljana, Slovenia*

* anze.bozic@ijs.si

## I. TOPOLOGICAL INDICES OF TREES AND CONNECTIONS BETWEEN THEM

### Trees and their topological indices

Given a tree $T$ with $N$ edges, we denote with $V(T)$ the set of its nodes and with $E(T)$ the set of its edges. We also introduce the Laplacian matrix of the tree, $\mathcal{L} = \mathcal{D} - \mathcal{A}$, where $\mathcal{D}$ is the degree matrix, a diagonal matrix of node degrees $d(i)$, $\mathcal{D} = \mathrm{diag}(d(i))$, and $\mathcal{A}$ is the adjacency matrix, a $(0,1)$-matrix where $\mathcal{A}_{ij} = 1$ if and only if nodes $i$ and $j$ are connected by an edge. The eigenvalues of the Laplacian matrix are denoted with $\lambda_i$, and the eigenvalues of the adjacency matrix with $\Lambda_i$.

Topological indices of a tree are numerical descriptors which characterize its topology. From the large amount of topological indices that have been introduced in graphs for various purposes [1–3], we have selected 18 commonly used ones, which we define below. We broadly divide them into five categories: *(i)* path-based indices which operate on the path lengths between nodes $\ell(i,j)$; *(ii)* degree-based indices which operate on node degrees $d(i)$; *(iii)* spectrum-based indices which operate on the eigenvalues of the Laplacian and adjacency matrices; *(iv)* centrality-based indices; and *(v)* information-based indices. For details and more indices, see Refs. [1–3] and references therein.

*Path-based indices*

- Wiener index:

$$W = \frac{1}{2} \sum_{i,j \in V(T)} \ell(i,j); \tag{S1}$$

- Maximum ladder distance (equivalent to graph diameter):

$$\mathrm{MLD} = \max_{i,j \in V(T)} \ell(i,j) \tag{S2}$$

and the related average ladder distance

$$\mathrm{ALD} = \frac{1}{N(N+1)} \sum_{i \neq j \in V(T)} \ell(i,j); \tag{S3}$$

- Balaban index (average distance-sum-connectivity index):

$$J = \frac{N}{N - |V(T)| + 2} \sum_{(i,j) \in E(T)} \Big[\ell(i)\ell(j)\Big]^{-1/2}, \tag{S4}$$

where $\ell(i) = \sum_{j \in V(T)} \ell(i,j)$ is the distance sum of the node $i$, and the prefactor is simplified to $N$ in the case of trees;

- Wiener polarity index:

$$P = \Big| \big\{ (i,j) \mid \ell(i,j) = 3,\ i,j \in V(T) \big\} \Big|. \tag{S5}$$

*Degree-based indices*

- Randić index:

$$R = \sum_{(i,j) \in E(T)} \Big[d(i)d(j)\Big]^{-1/2}; \tag{S6}$$

- First Zagreb index:

$$M_1 = \sum_{i \in V(T)} d(i)^2; \tag{S7}$$

- Second Zagreb index:

$$M_2 = \sum_{(i,j) \in E(T)} d(i)d(j); \tag{S8}$$

- Number of angles:

$$n_\theta = \frac{1}{2} \sum_{i \in V(T)} d(i)(d(i) - 1); \tag{S9}$$

- Atom-bond connectivity index:

$$\mathrm{ABC} = \sum_{(i,j) \in E(T)} \left[ \frac{d(i) + d(j) - 2}{d(i)d(j)} \right]^{1/2}; \tag{S10}$$

- Sum-connectivity index:

$$\mathrm{SC} = \sum_{(i,j) \in E(T)} \Big[d(i) + d(j)\Big]^{-1/2}. \tag{S11}$$

*Spectrum-based indices*

- Second and last Laplacian eigenvalue, $\lambda_2$ and $\lambda_N$;
- First-order network coherence:

$$H_1 = \frac{1}{2N}\sum_{i=2}^{N}\frac{1}{\lambda_i}; \tag{S12}$$

- Second-order network coherence:

$$H_2 = \frac{1}{2N}\sum_{i=2}^{N}\frac{1}{\lambda_i^2}; \tag{S13}$$

- Estrada index:

$$\mathrm{EE} = \sum_i e^{\Lambda_i}. \tag{S14}$$

*Centrality-based index*

- Balaban centric index:

$$B = \sum_i \delta_i^2, \tag{S15}$$

where $\delta_i$ is a sequence of numbers obtained by sequential tree pruning from its leaves towards its centre [4].

*Information-based index*

- Topological information content

$$I = \sum_i \frac{|\Omega_i|}{N+1}\log_2\left(\frac{|\Omega_i|}{N+1}\right), \tag{S16}$$

where the sum runs over all node orbits and $|\Omega_i|$ is the cardinality of orbit $\Omega_i$.

**Relationships between topological indices of trees**

For trees, there are several known relations between the indices in Eqs. (S1)–(S16). For instance, Wiener index $W$, a path-based index, can be related to the spectrum-based first-order network coherence $H_1$ [5],

$$W = 2N(N+1)H_1. \tag{S17}$$

Wiener polarity index $P$, another path-based index, can be shown to be a linear combination of first and second Zagreb indices, both degree-based [6]:

$$P = M_2 - M_1 + N \tag{S18}$$

Lastly, it can easily be shown that the number of angles $n_\theta$ is directly related to the first Zagreb index:

$$n_\theta = \frac{1}{2}M_1 - N \tag{S19}$$

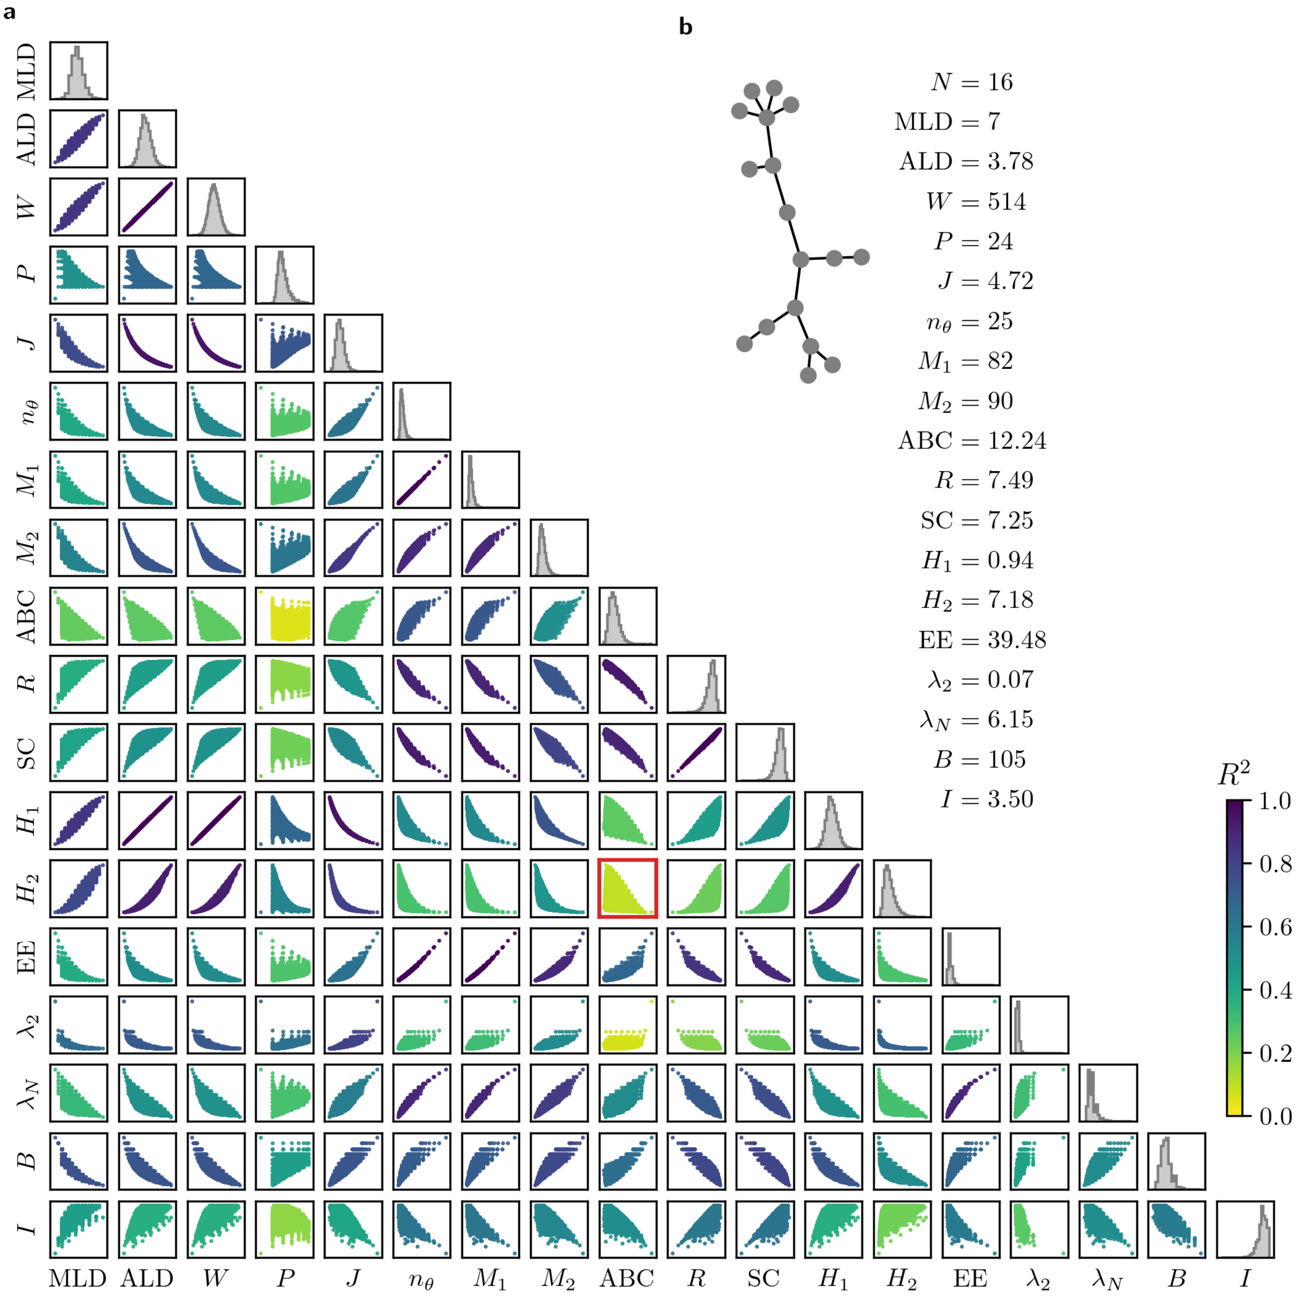


Figure S1. (**a**) Correlations between 18 different topological indices, calculated on all 48629 non-isomorphic trees with $N = 16$ edges. Colours correspond to the value of the correlation coefficient $R^2$. Diagonal elements show the distributions of individual indices. Highlighted plot shows the $(\mathrm{ABC}, H_2)$ space. (**b**) An example of a tree with $N = 16$ together with its values of topological indices.

**Extreme values and scaling of topological indices**

For most topological indices of trees, their minimum and maximum values are either the one of the linear or the star tree. They can often be determined analytically (Table S1), and they tend to scale non-linearly with tree size $N$ (Fig. S2).

| TI | Linear | Star | Minimum | Maximum |
|---|---|---|---|---|
| MLD | $N$ | $2$ | Star | Linear |
| ALD | $\frac{N+2}{3}$ | $\frac{2N}{N+1}$ | Star | Linear |
| $W$ | $\frac{1}{6}N(N+1)(N+2)$ | $N^2$ | Star | Linear |
| $P$ | $N-2$ | $0$ | Star[a] | N/A[b] |
| $J$ | $(N-2)\sum_{i=1}^{N-2}\frac{2}{2i^2-2Ni+(N-1)N}$ [c] | $\sqrt{\frac{N^3}{2N-1}}$ | Linear | Star |
| $n_\theta$ | $N-1$ | $\frac{1}{2}(N-1)N$ | Linear | Star |
| $M_1$ | $4N-2$ | $N(N+1)$ | Linear | Star |
| $M_2$ | $4(N-1)$ | $N^2$ | Linear | Star |
| ABC | $\frac{N}{\sqrt{2}}$ | $\sqrt{(N-1)N}$ | N/A[d] | Star |
| $R$ | $\frac{N}{2}+\sqrt{2}-1$ | $\sqrt{N}$ | Star | Linear |
| SC | $\frac{N}{2}+\frac{2}{\sqrt{3}}-1$ | $\frac{N}{\sqrt{N+1}}$ | Star | Linear |
| $H_1$ | $\frac{N+2}{12}$ | $\frac{N}{2N+2}$ | Star | Linear |
| $H_2$ | $\frac{1}{360}(N+2)(2N(N+2)+9)$ | $\frac{N^2+N-1}{2(N+1)^2}$ | Star | Linear |
| EE | $\sim I_0(2)N$ [e] | $N+2\cosh\left(\sqrt{N}\right)-1$ | Linear | Star |
| $\lambda_2$ | $2-2\cos\left(\frac{\pi}{N+1}\right)$ | $1$ | Linear | Star |
| $\lambda_N$ | $2-2\cos\left(\frac{\pi N}{N+1}\right)$ | $N+1$ | Linear | Star |
| $B$ | $(-1)^N\left((-1)^N(2N+1)-1\right)$ | $N^2$ | Linear | Star |
| $I$ | $\begin{cases}\log_2\left(\frac{N+1}{2}\right) & \text{odd } N\\ \log_2(N+1)-\frac{N}{N+1} & \text{even } N\end{cases}$ | $\log_2(N+1)-\frac{N\log_2(N)}{N+1}$ | Star | N/A |

[a] The *second smallest* value $P=N-2$ is obtained from the linear tree and general double-star trees [6].
[b] Maximum value of the index, $P=\lceil\frac{N-1}{2}\rceil\lfloor\frac{N-1}{2}\rfloor$, is obtained for certain types of trees with MLD $=3$ or MLD $=4$. See Ref. [7].
[c] The limit of this expression is $\pi$ as $N\to\infty$ [8].
[d] The study of extremal problem for the ABC index has proven to be difficult. Recently, a consistently tight lower bound has been proven for *chemical* trees [9].
[e] $\mathrm{EE(linear)}=\sum_{k=1}^{N+1}\exp\left(2\cos(k\pi/N)\right)\approx I_0(2)N-\cosh(2)$ [10]

Table S1. Analytical expressions for the values that the 18 topological indices used in our work assume for the linear and star trees. We also denote which tree assumes the minimum and maximum values for each index, where known.

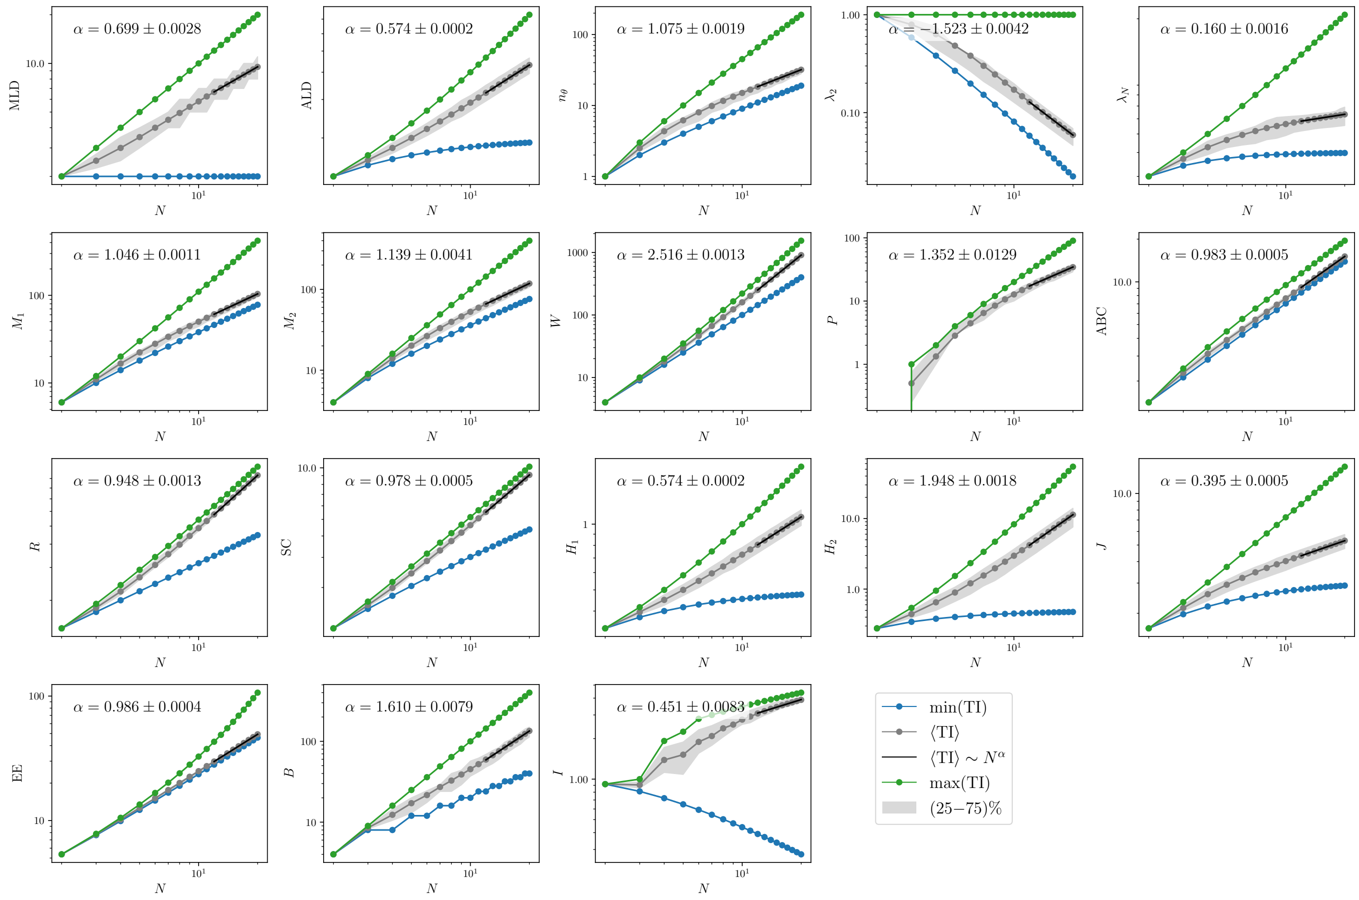

Figure S2. Scaling of the 18 topological indices analyzed in our work with increasing tree size $N$ for all non-isomorphic trees. Shown is the scaling of the two extreme values (cf. Table S1) and of the mean value of the index. Panel insets show the scaling exponents of the mean values, obtained through fits denoted by black lines.

## II. NORMALIZATION OF TOPOLOGICAL INDICES THROUGH THEIR CUMULATIVE DISTRIBUTION FUNCTIONS

Empirical distributions for different topological indices are selected from 101 different continuous distributions based on several criteria (see Methods in the main text). The fit parameters of the selected empirical distributions at different tree sizes $N$ are then estimated using maximum likelihood estimation method on the distribution of an index over 10000 random trees (panels (a)–(d) of Fig. S3). Afterwards, we fit the dependency of each distribution parameter $p$ on the tree size $N$ with a power-law model $p = \alpha x^{\beta}$ (panels (e)–(h) of Fig. S3). The only exception to this is the parameter $\kappa$ in Pearson type III distribution for $W$, which is fitted using an inverse law $\kappa = \alpha/x + \beta$. Figure S4 furthermore shows that sampling the values of a topological index on 10000 random trees is sufficient to obtain a good approximation to the distribution of a topological index over the space of all (non-isomorphic) trees.

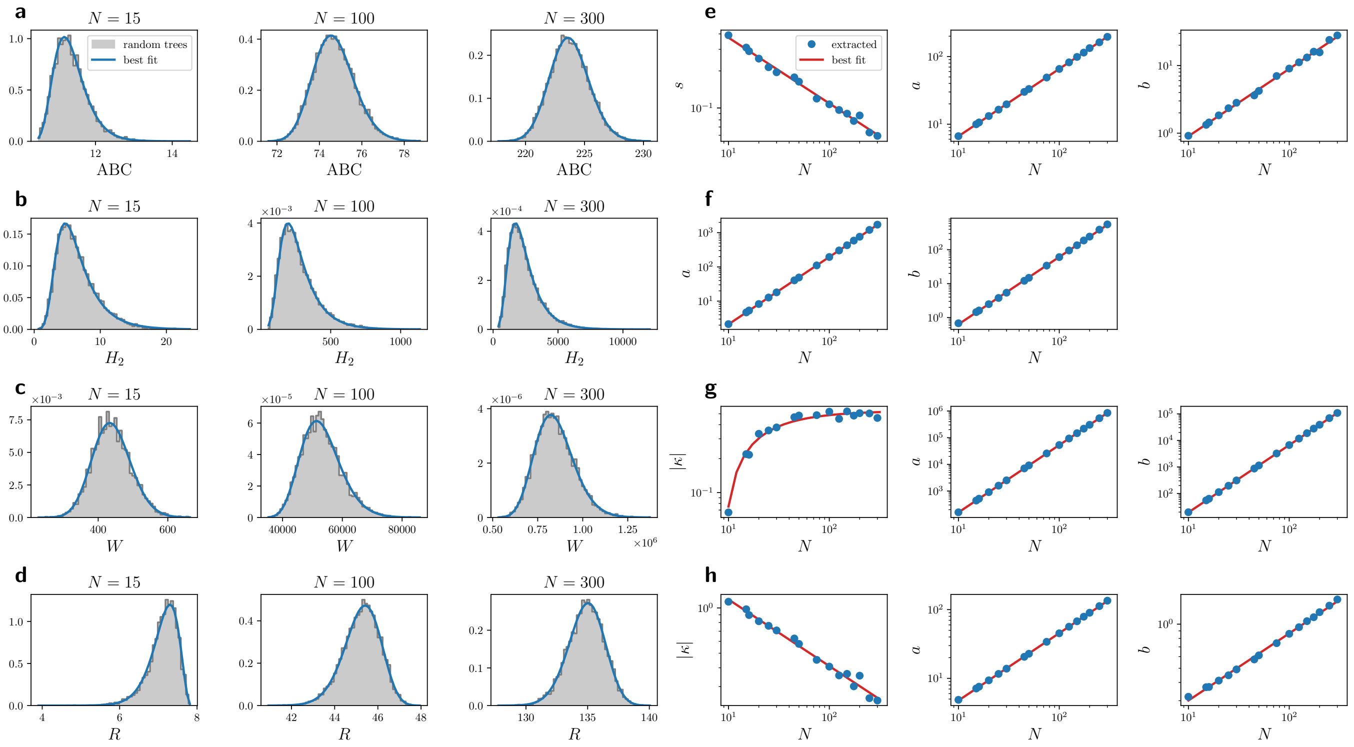


Figure S3. **(a–d)** Empirical distributions of four topological indices to sets of 10000 random trees at three different tree sizes $N$ and fitted analytical distributions (see Methods). (a) Second-order network coherence $H_2$, (b) atom bond connectivity index ABC, (c) Randić index $R$, and (d) Wiener index $W$. **(e–h)** Extracted parameters $p$ of fit of the empirical distributions of the four topological indices to the analytical distributions at various $N$. Lines show the fitted power-law scaling of the fit parameters with tree size $N$, $p = \alpha N^{\beta}$. The exception is the fit parameter $\kappa$ for $W$, where inverse-law $|\kappa| = \alpha/x + \beta$ is used instead of the power law.

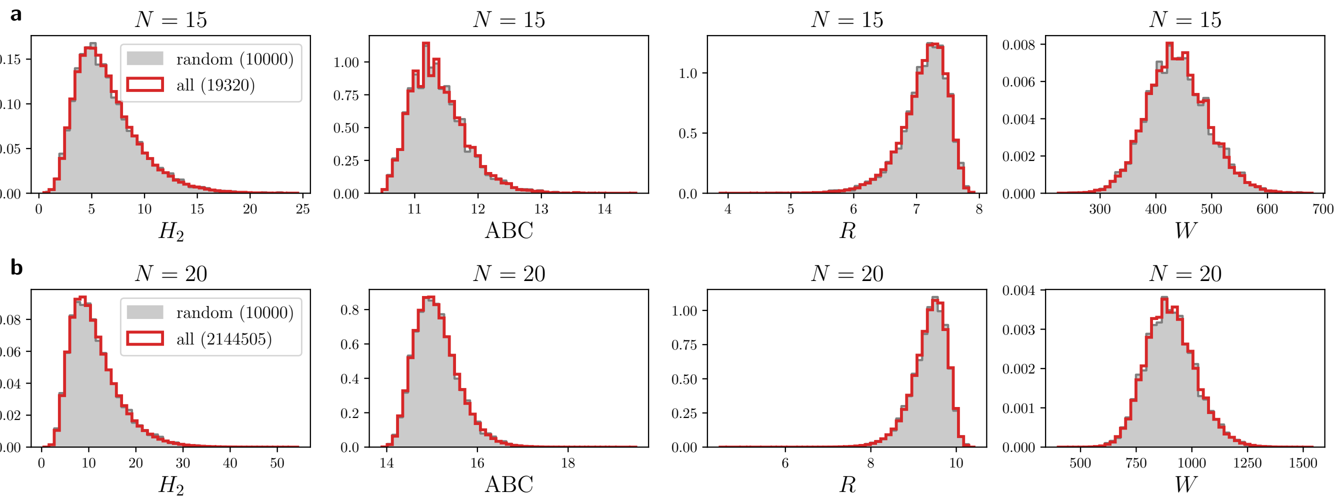


Figure S4. Distributions of four topological indices (second-order network coherence $H_2$, atom bond connectivity index ABC, Randić index $R$, and Wiener index $W$) on set of 10000 random trees and on the whole set of non-isomorphic trees for **(a)** $N = 15$ and **(b)** $N = 20$.

# III. CHARACTERIZATION OF $(\mathrm{ABC}^*, H_2^*)$ SPACE

## Special tree topologies at the phase space boundary

In Fig. 2 in the main text, we show that the upper boundary of the $(\mathrm{ABC}^*, H_2^*)$ space consists of star-like trees while the lower and right boundaries consist of dumbbell trees. Figure S8 shows how these two types of trees are defined and generated as a function of generating parameter $k$ on an example of trees with $N = 16$. Going from a star tree ($k = 0$) to a spider tree ($k = \lfloor N/2 \rfloor$) involves removing individual leaves from the star tree and attaching them to others, forming branches of length 2 in the process (Fig. S8a). Going from a linear tree ($k = N - 3$) to a short dumbbell ($k = 1$) involves removing interior edges and attaching them to the end of the tree with fewer branches (Fig. S8b).

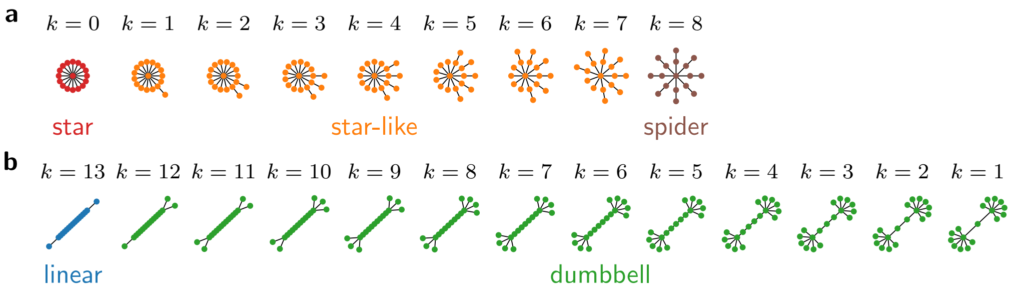


Figure S5. Construction of special tree topologies found at the boundary of $(\mathrm{ABC}^*, H_2^*)$ space, demonstrated on an example of trees with $N = 16$. **(a)** Star-like trees, progressing from star tree at $k = 0$ to spider tree at $k = 8$ and **(b)** dumbbell trees, progressing from linear tree at $k = 13$ to shortest dumbbell at $k = 1$. See also Fig. 2 in the main text.

## Discriminative power of ABC and $H_2$

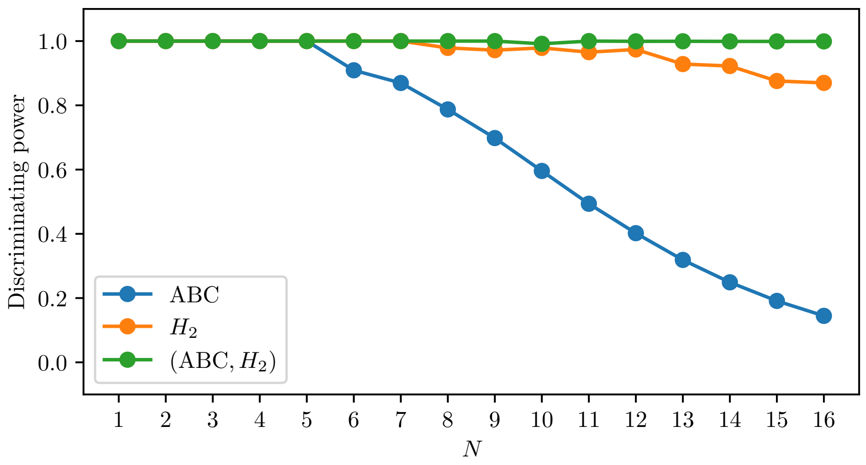


Figure S6. Discriminative power of topological indices ABC, $H_2$, and their pair $(\mathrm{ABC}, H_2)$. Discriminative power denotes the fraction of unique values of a topological index, determined here over the space of all non-isomorphic trees at various tree sizes $N$.

### Fraction of trees with negative values of ABC$^*$

Atom bond connectivity index, ABC, is one of the few indices we examined whose minimum value is not one of either the linear or the star tree (Table S1). By nonetheless normalizing the index ABC$^*$ in such a manner that ABC$^*$(linear) $= 0$ [Eq. (5) in the main text], we are left with a small fraction of trees at each tree size $N$ that have ABC$(T) <$ ABC(linear) or, equivalently, ABC$^*(T) < 0$. Figure S7 shows that this fraction is negligible and tends steeply towards zero for tree sizes larger than $N \gtrsim 30$.

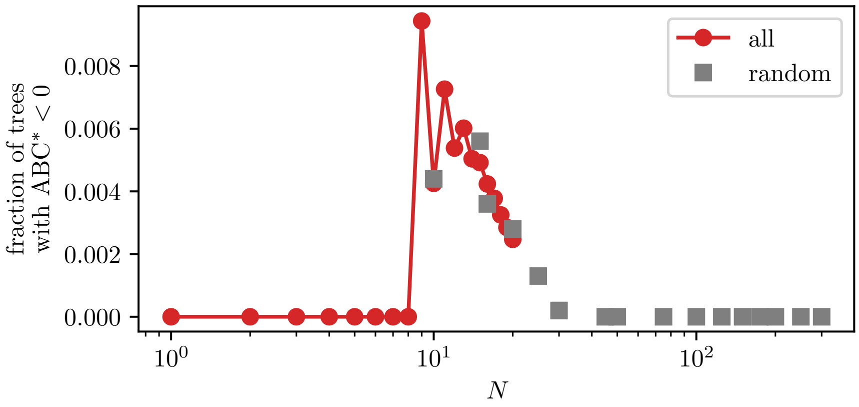


Figure S7. Fraction of trees with ABC$^* < 0$ as a function of tree size $N$. For small enough trees (i.e., $N \leq 20$), the fraction is evaluated on all non-isomorphic trees. For larger tree sizes, the fraction is determined on a sample of 10000 random trees.

### Properties of (ABC$^*, H_2^*$) space

Figure 2g in the main text shows that chemical trees—trees with maximum node degree 4—and caterpillar trees—trees where all the nodes are within distance 1 of a central path—occupy different parts of the (ABC$^*, H_2^*$) space. Panels (a) and (b) of Fig. S8 show that the part of the phase space that these trees occupy furthermore shrinks as the tree size $N$ is increased. Panels (c) and (d) of Fig. S8 then show how the maximum node degree and the fraction of degree 2 nodes change in the space of all (non-isomorphic) tree topologies. We also employ four different tree transformations on four randomly chosen trees with $N = 50$ and study where the transformed trees lie in the phase space (panels (e)–(h) of Fig. S8). Namely, we use:

- Random leaf remove: A randomly selected leaf (degree 1 node) is removed;
- Random leaf move: A randomly selected leaf (degree 1 node) is removed and a new leaf is added to a randomly selected node in a tree;
- Prüfer shuffle: The Prüfer sequence of a tree is randomly shuffled, leading to a tree with a same distribution of node degrees $d(i)$ but a different topology (see, e.g., Refs. [11, 12]);
- Random subtree swap: A randomly selected edge is removed, resulting in two disconnected trees; a new edge is then added between two randomly selected nodes of the two trees to form a new tree.

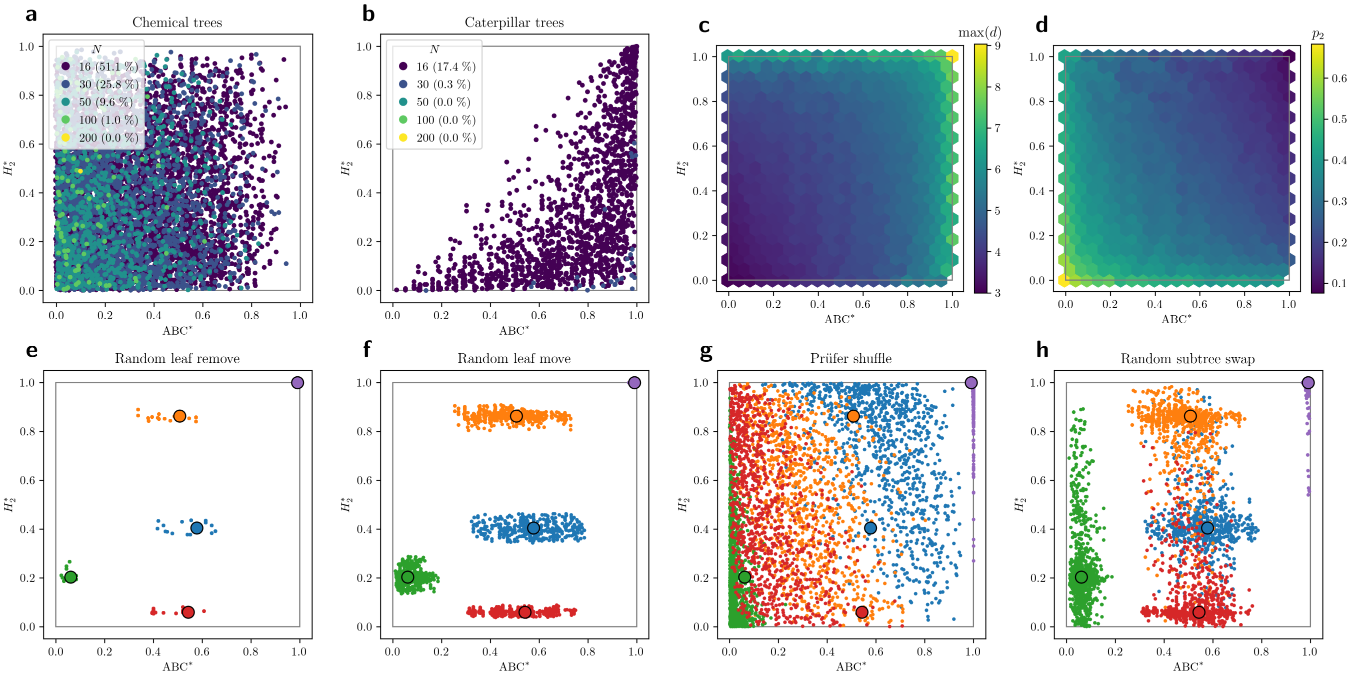


Figure S8. Characterization of the $(\mathrm{ABC}^*, H_2^*)$ space. Changes in the proportion of **(a)** chemical and **(b)** caterpillar trees in the phase space with increasing tree size $N$, estimated from a sample of 10000 random trees. Heatmaps of **(c)** maximum node degree and **(d)** fraction of degree 2 nodes for trees of size $N = 16$. Changes in the $(\mathrm{ABC}^*, H_2^*)$ space for trees with $N = 50$ upon performing four different types of tree transformations 1000 times on five randomly chosen trees (black circles): **(e)** random leaf move, **(f)** random leaf remove, **(g)** Prüfer shuffle and **(h)** random subtree swap. See the text for more details on these transformations.

## IV. MAPPING RNA SECONDARY STRUCTURE TO A TREE

We employ two different methods of mapping a secondary structure of RNA to a tree (see Methods in the main text and Fig. S9). Roughly speaking, the first, simple method treats every presence of an unpaired nucleotide as a node, hence giving a tree with more nodes (Fig. S9b), while the second, RAG-based method is more conservative and gives a more "coarse-grained" representation of the structure (Fig. S9d).

It should be noted that the rules of RAG method (and its online implementation) occasionally lead to disjoint graphs and not trees, which occurs when the RNA structure includes a multiloop with no unpaired nucleotides (see Fig. S9c). To alleviate this issue, we always first generate a tree with the simple method and then use a sequence of node contractions and deletions to convert this tree to the RAG-based method while relaxing the 1$^{st}$ rule for multiloops.

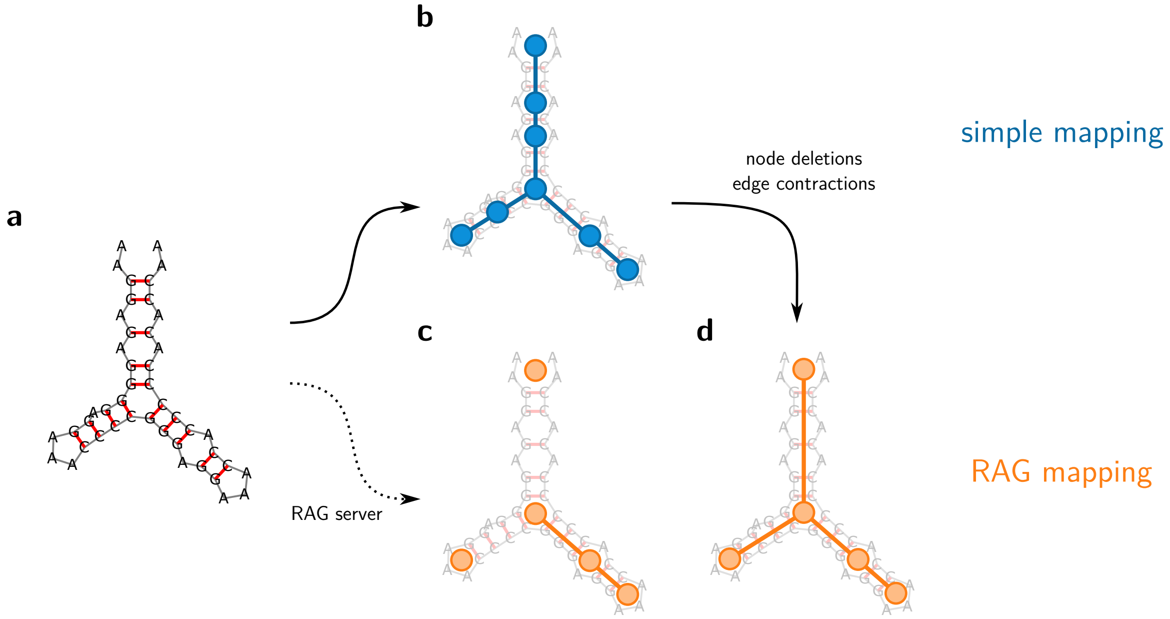


Figure S9. Mapping an RNA structure to a mathematical tree in two different ways. **(a)** Example RNA structure of 45 nucleotides with nucleotide sequence `AAGGAGAGGGGAGGAAACCCCGGGAGGAAACCACCCCCACACCAA` and dot-bracket structure `..((.(.((((.((...))))(((.((...)).)))))).).))...` **(b)** Simple method of mapping an RNA structure to a tree. **(c)** RAG-based method of mapping an RNA structure to a tree. Due to the presence of a multiloop with no unpaired nucleotides, in this case the method leads to a disconnected graph and not to a tree. **(d)** Modified RAG-based method of mapping an RNA structure to a tree which correctly yields a tree (see text for details).

## V. METHODS OF COARSE-GRAINING TREES

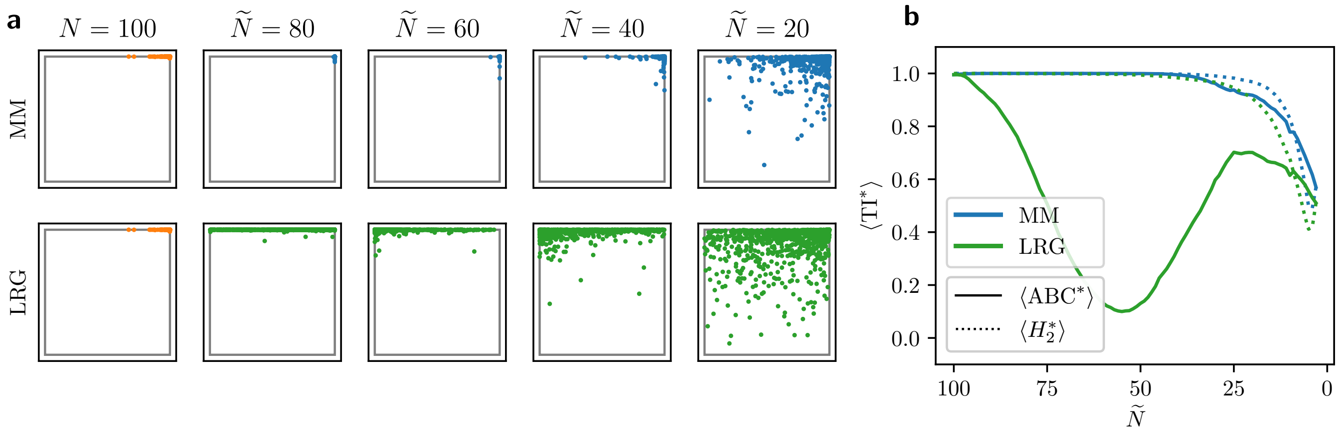


Figure S10. Effects of MM and LRG tree coarse-graining methods on scale-free Barabási-Albert (BA) trees (cf. also Fig. 4 in the main text). **(a)** Phase space flow of $10^3$ random BA trees upon their coarse-graining from $N = 100$ to progressively smaller target $\widetilde{N}$ using either MM (top row) or LRG (bottom row) coarse-graining. **(b)** Changes in the average values of normalized topological indices $\langle \mathrm{ABC}^* \rangle$ and $\langle H_2^* \rangle$ with the size of coarse-grained trees $\widetilde{N}$ using the MM and LRG methods. The values of the two indices are averaged over 1000 random BA trees.

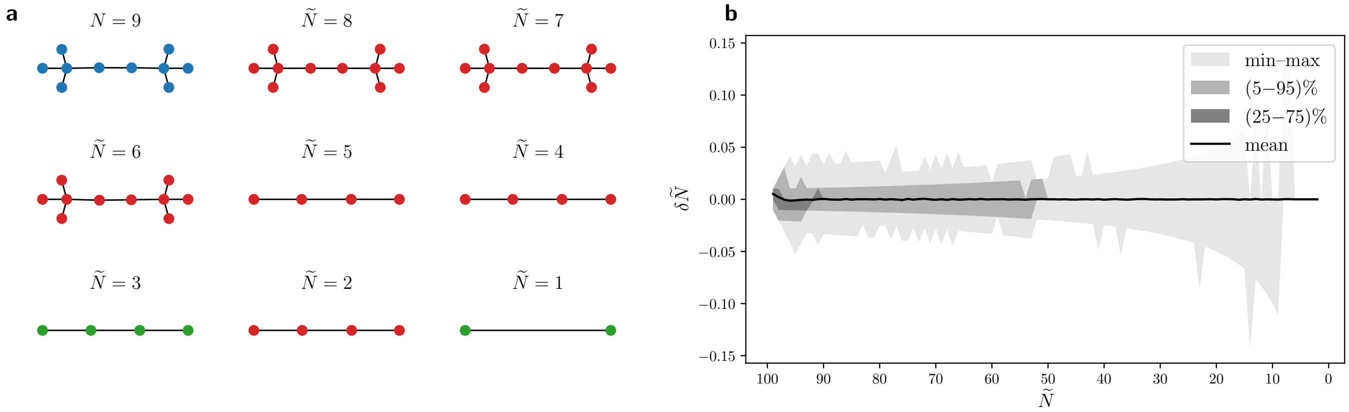


Figure S11. **(a)** Example of a tree with $N = 9$ edges which can be coarse grained using the LRG method only to $N_{\mathrm{actual}} = 3$ or $N_{\mathrm{actual}} = 1$ depending on the target $\widetilde{N}$. **(b)** Distribution of the relative error $\delta\widetilde{N} = (N_{\mathrm{actual}} - \widetilde{N})/\widetilde{N}$ when coarse-graining 1000 random trees with $N = 100$ to various $\widetilde{N}$.

## VI. EXTENDING $(\mathrm{ABC}, H_2)$ SPACE TO GRAPHS

In order to see how the $(\mathrm{ABC}, H_2)$ space changes if we calculate the two indices on *graphs* instead of trees, we generated sets of all unicyclic, bicyclic and tricyclic graphs (i.e., graphs having the cyclomatic number $|E(G)|-|V(G)|+1$ equal to 1, 2, or 3). These were generated using `geng` function from nauty 2.8.8 [13]. The resulting phase space and the distributions of the values of individual indices are shown in Fig. S12.

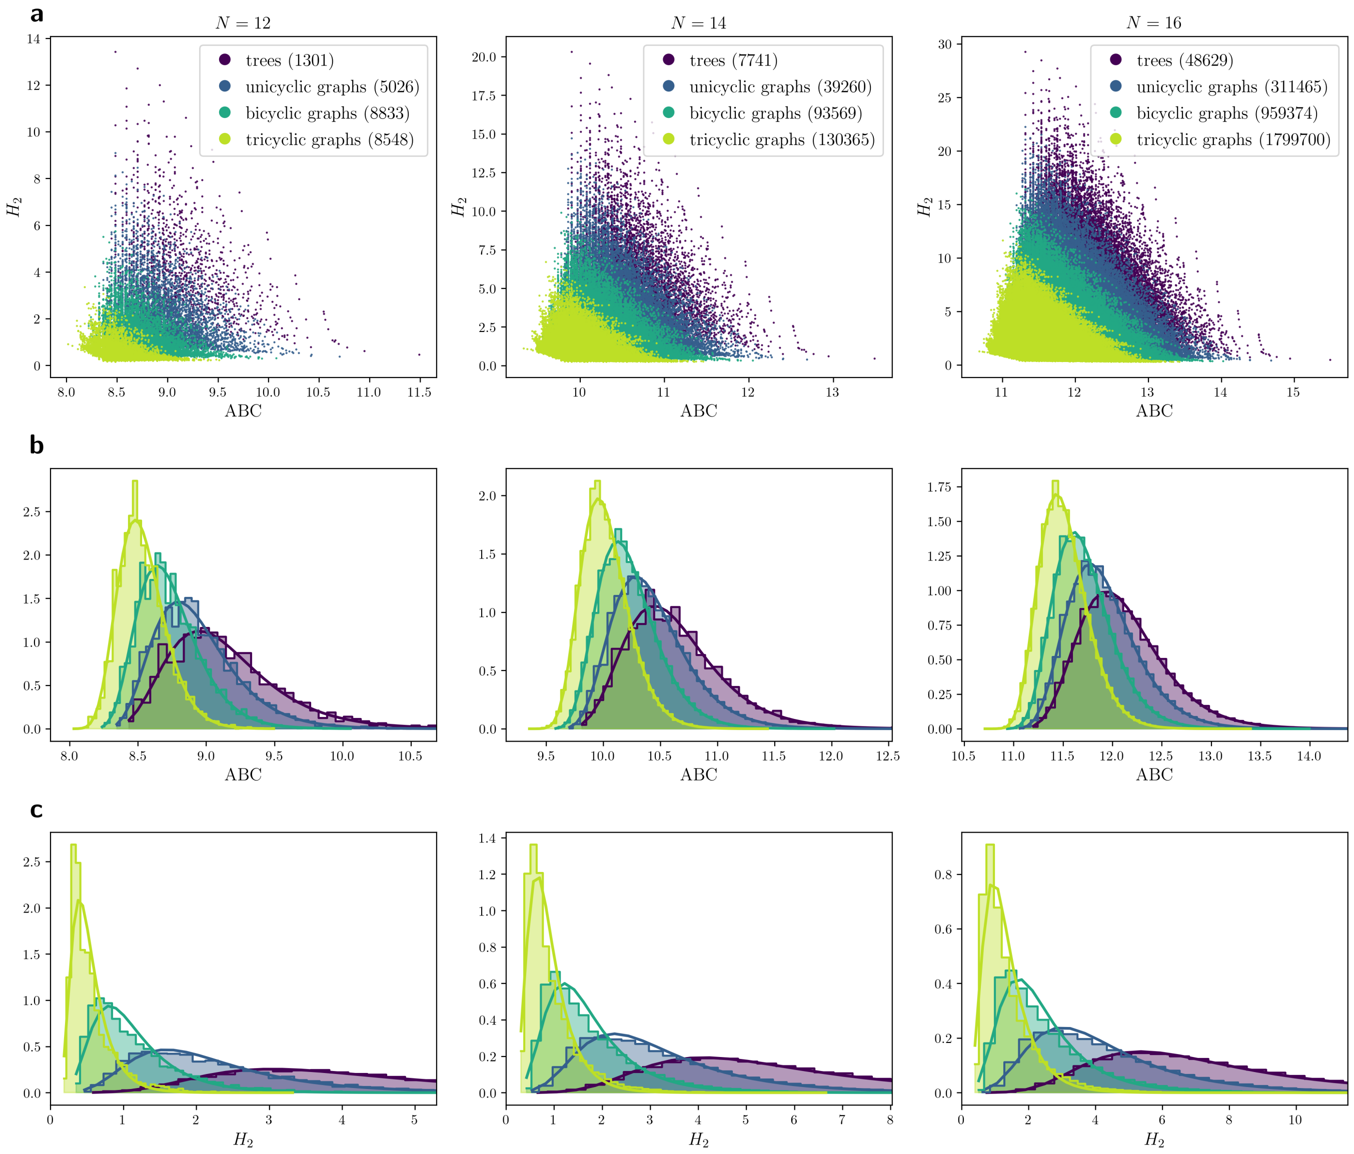


Figure S12. **(a)** Non-normalized $(\mathrm{ABC}, H_2)$ space for the sets of all trees and all unicyclic, bicyclic, and tricyclic graphs having the same number of edges $N$. The numbers in brackets denote the number of trees or graphs in each group. Fits to the distributions of **(b)** ABC (log-normal distribution) and **(c)** $H_2$ (Moyal distribution).

## VII. PHASE SPACE CONSTRUCTED WITH WIENER AND RANDIĆ INDICES

Figure S13 shows the example of a both non-normalized and normalized phase space constructed using two topological indices other than the ones in the main text, namely Wiener index $W$ and Randić index $R$. The distributions for both are estimated using Pearson type III distribution,

$$f(x;\kappa,a,b) = \frac{|\beta|}{b\,\Gamma(\alpha)}\left(\beta\left(\frac{x-a}{b}-\zeta\right)\right)^{\alpha-1}\exp\left(-\beta\left(\frac{x-a}{b}-\zeta\right)\right), \tag{S20}$$

with $\beta = 2/\kappa$, $\alpha = \beta^2 = 4/\kappa^2$, and $\zeta = -\alpha/\beta = -2/\kappa$. This distribution forms the basis for their normalization, which follows the definition in Eq. (5) in the main text.

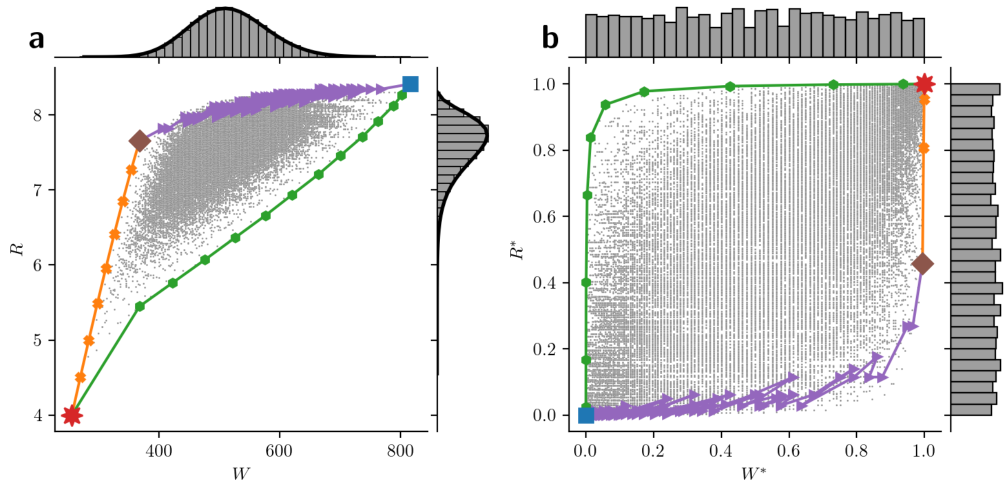


Figure S13. Phase space obtained using Wiener index $W$ and Randić index $R$. **(a)** Non-normalized $(W, R)$ space and **(b)** normalized $(W^*, R^*)$ space for all trees with $N = 16$. Coloured phase space boundaries correspond to the same trees as in Fig. 2b in the main text.

## SUPPORTING REFERENCES

[1] A. Balaban, I. Motoc, D. Bonchev, and O. Mekenyan, Topological indices for structure-activity correlations, in *Steric effects in drug design* (Springer, 1983) pp. 21–55.
[2] I. Gutman, Degree-based topological indices, Croat. Chem. Acta **86**, 351 (2013).
[3] M. I. Stankevich, I. V. Stankevich, and N. S. Zefirov, Topological indices in organic chemistry, Russ. Chem. Rev. **57**, 191 (1988).
[4] A. T. Balaban, Chemical graphs: XXXIV. Five new topological indices for the branching of tree-like graphs, Theor. Chim. Acta **53**, 355 (1979).
[5] B. Mohar, D. Babic, and N. Trinajstic, A novel definition of the wiener index for trees, J. Chem. Inf. Comput. Sci. **33**, 153 (1993).
[6] M. Liu and B. Liu, On the wiener polarity index, MATCH Commun. Math. Comput. Chem **66**, 293 (2011).
[7] W. Du, X. Li, and Y. Shi, Algorithms and extremal problem on Wiener polarity index, Match **62**, 235 (2009).
[8] A. Balaban, N. Ionescu-Pallas, and T. Balaban, Asymptotic values of topological indices $J$ and $J'$ (average distance sum connectivities) for infinite cyclic and acyclic graphs, MATCH Commun. Math. Comput. Chem **17**, 121 (1985).
[9] W. Gao, The minimum abc index of chemical trees, Discrete Appl. Math. **348**, 132 (2024).
[10] I. Gutman and A. Graovac, Estrada index of cycles and paths, Chem. Phys. Lett. **436**, 294 (2007).
[11] S. W. Singaram, A. Gopal, and A. Ben-Shaul, A prufer-sequence based algorithm for calculating the size of ideal randomly branched polymers, J. Phys. Chem. B **120**, 6231 (2016).
[12] D. Vaupotič, A. Rosa, L. Tubiana, and A. Božič, Scaling properties of RNA as a randomly branching polymer, J. Chem. Phys. **158** (2023).
[13] B. D. McKay and A. Piperno, Practical graph isomorphism, ii, J. Symb. Comput. **60**, 94 (2014).
